# Supplementary material for: Toward Deep Learning Based Access Control
Source: arXiv:2203.15124 source file (2022-03-28)
Supplement: Supplementary file 1 [file appendices.tex]

\appendix

\section{Improving FPR Performance}
\label{app:fprImprovement}

\begin{table}
\centering
\scriptsize
  \caption{Different Combination of Weight for Different Classes for the Loss Function.}
  \label{tab:weightLossCombination}
  \resizebox{0.9\linewidth}{!}{%
  \begin{tabular}{ccc}
    \hline
    Combination Name
    & Grant Class Weight
    & Deny Class Weight
    \\\hline
    equal weight & 1.0 & 1.0 \\
    wlc-1 & 0.07 & 0.93 \\
    wlc-2 & 0.03 & 1.0 \\
    wlc-3 & 0.01 & 0.8 \\
    wlc-4 & 0.01 & 1.0 \\
    \hline
  \end{tabular}
  }
\end{table}

\begin{figure}[ht]
    \centering
	\includegraphics[width=\linewidth]
	{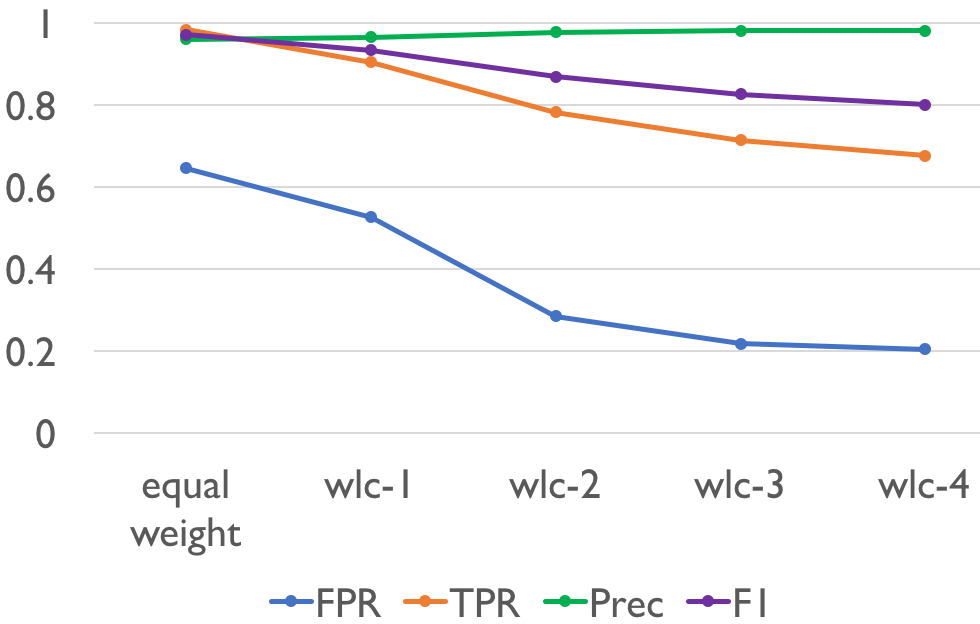}
	\caption{FPR Performance Improvement in \(\DLBACALPHA\).}
	\label{fig:fprImprovemnt}
\end{figure}

This section shows how to improve False Positive Rate (FPR) performance in \(\DLBACALPHA\). We apply a well-known technique for performance improvement (or control) of an imbalanced dataset. The idea is to give more weight to the wrong prediction for samples from minority classes and vice-versa. However, improving in one metrics might affect the other performances.
We experiment with \(\DLBACALPHAD\) instance for the \(\AMAZONKAGGLE\) dataset where there are two different classes for each sample, deny and grant.
In the \(\AMAZONKAGGLE\) dataset, there are only below 7\% of the samples from denying class. Hence, we modify the loss function while training the \(\DLBACALPHAD\) to add majority weights on loss for the deny class and significantly smaller weights for the other one. 
As reported in Table~\ref{tab:weightLossCombination}, we consider four different combinations of weight for the loss function for different classes.
Figure~\ref{fig:fprImprovemnt} showed, with the weight decrease for the grant class and increased weight for the deny class, the FPR reduces. It also positively impact precision which rises consistently. However, the F1 score and TPR are also affected and decrease gradually.

\section{Impact of Metadata with Non-significant Attribution Scores}
\label{app:impactNonSignificantMetadata}
To understand the effect of the metadata having non-significant or low attribution scores from Integrated Gradients, we take the attribution scores for the tuple that we presented in Figure~\ref{fig:modifyAccessThroughIG} (tuple2). There we see that the user Carol has \emph{deny} access to the projectC resource for op1 operation. We take the attribution scores for the Carol and projectC tuple and, as illustrated in Figure~\ref{fig:denyAccessTupleInterpretation}, the rmeta2 and umeta2 are the most influential metadata with the highest attribution scores. However, umeta4, umeta5, rmeta0, rmeta3, rmeta5 metadata have 0.0 attribution scores, which indicates that they have no impact on this specific decision, whereas rmeta7 and umeta7 (along with some other metadata) have less influence (smaller attribution scores). We want to evaluate the consequence if we change the value of these non or less significant metadata. We modify the value of all these metadata and replace it with the value of a known tuple (Dave and projectD) with grant access. We found no change in the access decision.

\begin{figure}[t]
    \centering
	\includegraphics[width=\linewidth]
	{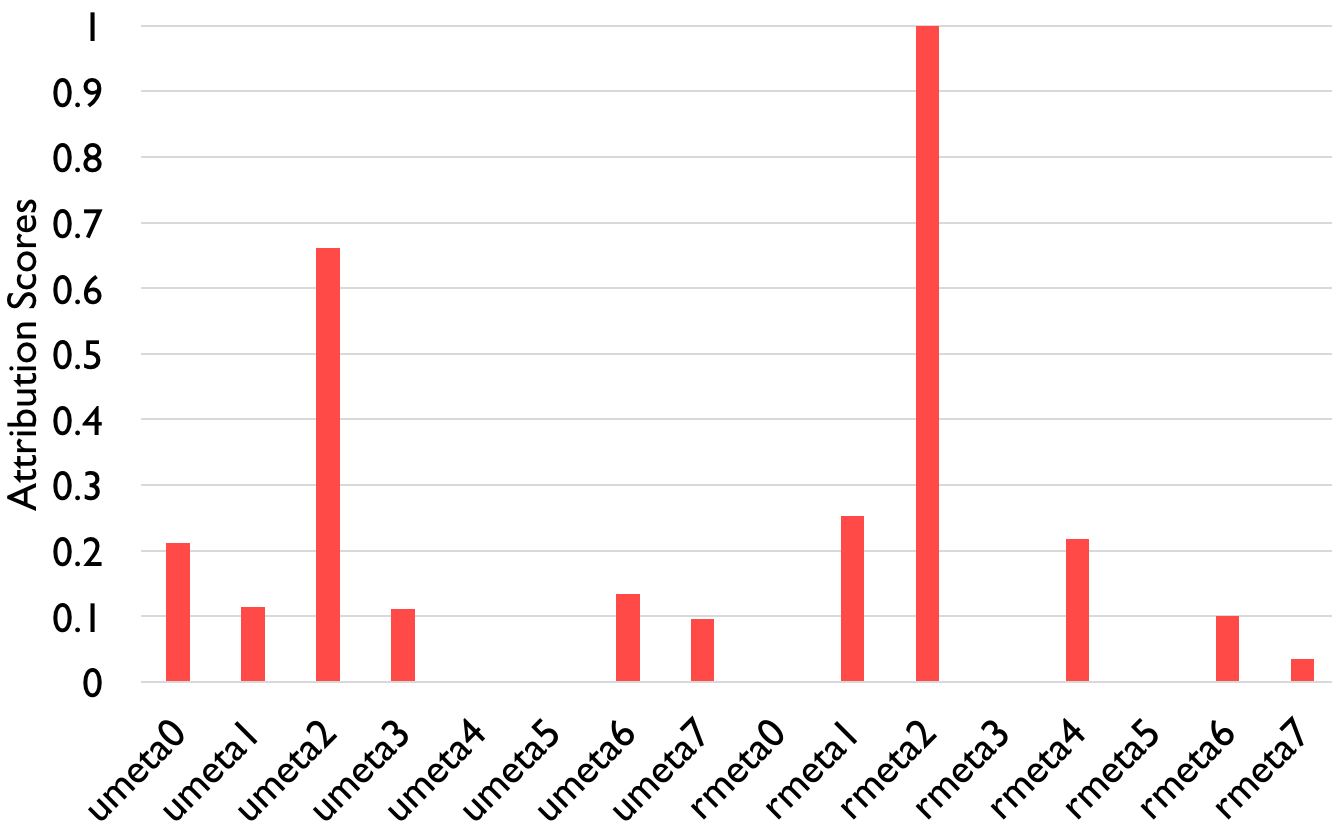}
	\caption{Local Interpretation of a Tuple with Deny Access.}
	\label{fig:denyAccessTupleInterpretation}
\end{figure}

\section{Decision Tree for Knowledge Transferring}
\label{app:decisionTree}

\begin{figure*}[t]
    %\centering
	\includegraphics[width=0.8\textwidth]
	{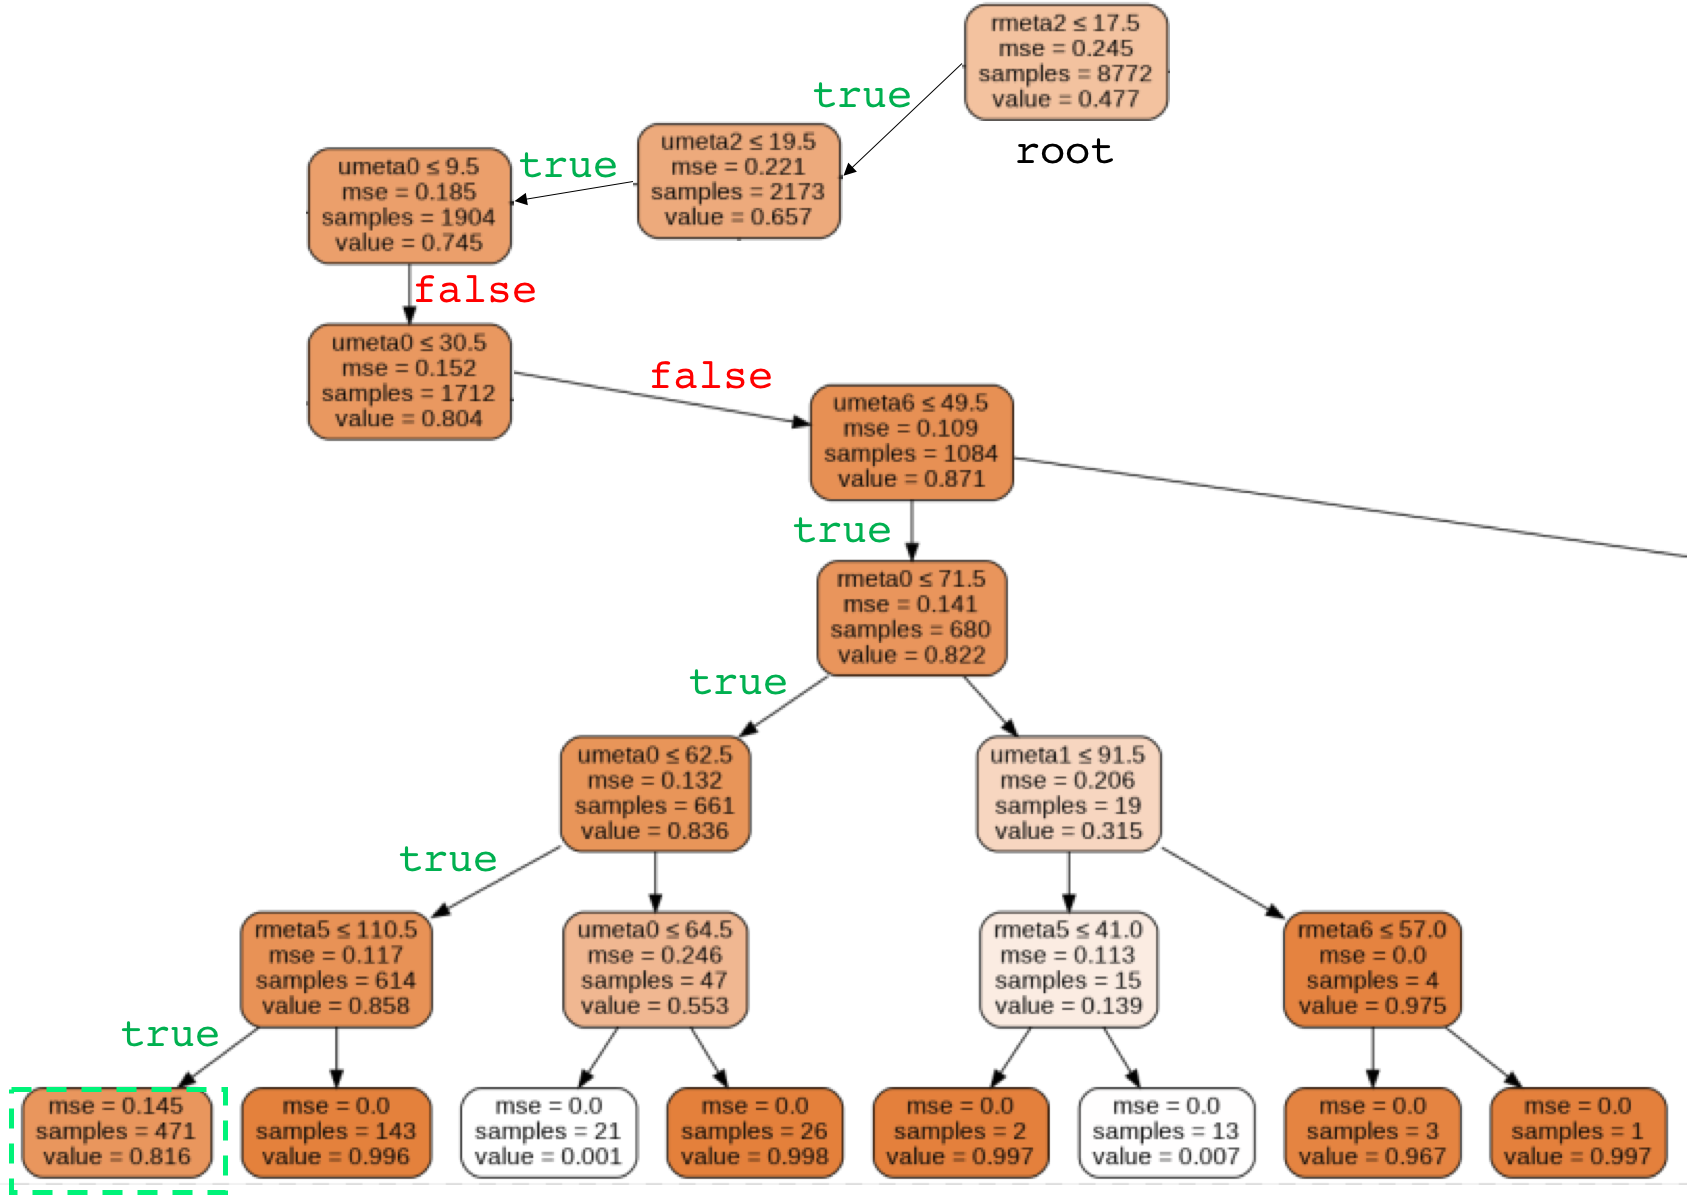}
	\caption{Decision Tree Generated for \(\SMALLA\) Dataset. Part of the tree has been cropped for better illustration.}
	\label{fig:decisionTree}
\end{figure*}

We build a decision tree for (\(\SMALLA\)) dataset and \emph{op1} operation. We train the tree based on the training data that contain both user-resource metadata and their corresponding access permission for \emph{op1} operation. However, instead of giving permissions from the dataset, we provide corresponding \emph{probabilities} acquired from \(\DLBACALPHA\). We accumulate \textit{op1} access \textit{probabilities} for the tuples in (\(\SMALLA\)) dataset, as discussed in Section~\ref{knowledgeTransferring}. Then we train the decision tree based on the training input from the dataset and probabilities as the target output (ground truth).

Figure~\ref{fig:decisionTree} is the decision tree generated from the \(\SMALLA\) dataset (with 8772 samples) based on \emph{Knowledge Transferring} for \emph{op1} operation. We demonstrate how to retrieve a rule from the tree to understand any specific decision. We cropped the tree for better visualization. Each node in the tree represents a binary decision point where the samples are split based on the condition in the corresponding node. For example, the tree's root node is rmeta2 that splits all the 8772 samples based on the `rmeta2$<=$17.5' condition. 
As specified, the metadata values of our datasets are categorical, where values are integer representations of different categories. Therefore, we can round the value in each node's condition to the next integer without any issue. For instance, we can round the value of rmeta2$<=$17.5 to rmeta2$<$18 as there is no metadata value of 17.5. The MSE (mean-squared error) indicates the error that measures the quality of a split. Also, the value of the node determines the probabilities for related decisions. As we build this tree for \emph{op1} operation, we have a binary decision point --- whether or not the user has access to the corresponding resource for this operation. We round the probabilities to the \emph{grant} if the value is $>$0.5, otherwise \emph{deny}. As shown in the figure, the value in the root node is 0.478 indicates that initially, all the requests are considered `denied'.

%The Figure~\ref{fig:decisionTree} is decision tree generated from the \(\SMALLA\) dataset based on \emph{Knowledge Transferring} for \emph{op1} operation. We demonstrate how to retrieve a rule from the tree to understand any specific decision. We cropped the tree for better visualization. Each node in the tree represents a binary condition (top of each node, e.g., rmeta2$<=$17.5) for a metadata. The following node will be the left node if the condition is true, right node otherwise. Also, the value of the node determines the probabilities for related decisions. As we build this tree for \emph{op1} operation, we have a binary decision point --- whether or not the user has access to the corresponding resource for this operation. We round the probabilities to the \emph{grant} if the value is $>$0.5, otherwise \emph{deny}. The label samples in the node indicate the number of samples affected based on the corresponding condition, and mse (mean-squared error) indicates the error that measures the quality of a split.
%We see the root node of the tree is rmeta2. Recall that we found \emph{rmeta2} as the most significant metadata for this dataset according to our global interpretation in Section~\ref{integratedGradients}. As our metadata are categorical (values are integer representation of a category), we can consider each condition to the next integer. For example, we can consider the condition rmeta2 $<=$ 17.5 as rmeta2 $<$ 18.

We will walk through an access request for user \emph{Dave}'s access to the \emph{projectD} resource for \emph{op1} operation as described in Section~\ref{knowledgeTransferring}. The metadata value of Dave and projectD is available in Figure~\ref{fig:modifyAccessThroughIG} (tuple1). However, the value of rmeta2 metadata is 5 for \emph{projectD}; hence the root condition is true, and the next node is the left node with condition umeta2$<$20. This condition is also successful for Dave's umeta2$=$5 and checks the next left node to see the value of umeta0. As the value of umeta0 is 61, it can directly come to the node where umeta6 is verified. This condition is passed with umeta6$=$6, and the next left condition is also satisfied for the rmeta0$=$30. The following condition is true as the value of umeta0 is 61. Finally, the tree checks for the value of rmeta5 before making the access decision for \emph{Dave} to the \emph{projectD}. This condition is also successful for rmeta5$=$105.
We see the green shaded node is the final decision node for this request. The decision is \emph{grant} based on the value 0.82 ($>$0.5).
